# Supplementary material for: Rattling mode and symmetry lowering resulting from instability of B$_{12}$-molecule in LuB$_{12}$
Source: arXiv:1707.06516 source file (2017-07-20)
Supplement: Supplementary file 1 [file SupplInf.pdf]

**Supplementary Information.**

**Experimental details.** Single crystals of lutetium dodecaboride were grown by induction zone melting in an inert gas atmosphere. Structural studies were carried out on the X-ray diffractometer Xcalibur (MoK$\alpha$-radiation, graphite monochromator) [S1]. Measurements of the transverse magnetoresistance and the Hall effect were performed in a five-terminal scheme with a direct current at temperatures in the range 1.8-300 K in a magnetic field up to 80 kOe with the help of installation with a sample rotating in a magnetic field [S2]. Precise X-ray diffraction reflexes (Fig. S1) and quantum oscillations of the magnetization (de Haas-van Alphen effect) obtained in the orientation of the magnetic field ***H*** || [100] (Fig. S2), testify to the high quality of crystals under investigation.

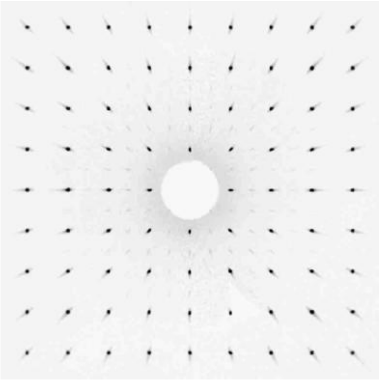

**Fig.S1.** The $l$=0 plane of the $LuB_{12}$ diffraction pattern.

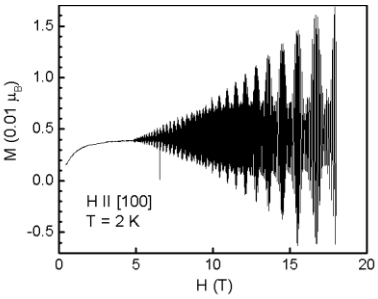


**Fig.S2.** de Haas- van Alphen oscillations obtained in the orientation of the magnetic field ***H*** || [100].

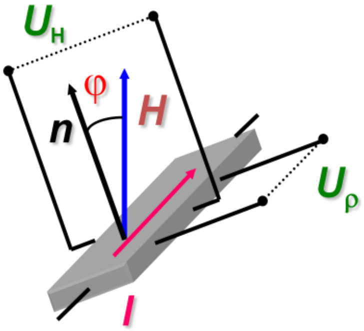


**Fig.S3.** Measuring scheme of magnetoresistance and Hall effect with the sample rotating about the current axis **I** (pink line); $U_\rho$ and $U_H$ are resistance and Hall voltages.

**Fine details of atomic structure.** Structure symmetry of $LuB_{12}$ (Fig.1a-b in the paper) is presented in literature by cubic *Fm*-3*m* group. Some problems appear, however, how the cubic symmetry of the structure can be adjusted to significant anisotropy of magnetoresistance observed in this work. Fine details of atomic structure, which may be lost in the high-symmetrical structural

model, can be derived from residual electron density (ED) distribution taking difference Fourier maps into consideration. Fourier synthesis of ED is a computational procedure, which starts with a set of both experimental and previously calculated parameters. Computational formula can be written in general terms as follows (see, for instance, the Fourier procedure in the user manual of Jana program [S3]:

$$G(\mathbf{r}) = (1/V)\Sigma_{\Delta\mathbf{S}}\, A(\mathbf{\Delta S})\exp[i\varphi(\mathbf{\Delta S})]\, \exp(-2\pi i\, \mathbf{\Delta S}\cdot\mathbf{r}) \quad (1)$$

Here $G(\mathbf{r})$ is either ED ($g$) or residual ED ($\Delta g$) resulting either from a 'regular' or difference Fourier synthesis, respectively;

$V$ is a unit-cell volume;

$\mathbf{\Delta S} = \mathbf{S} - \mathbf{S}_0 = \Sigma\, h_i\, \mathbf{a}^*_i$ – a Bragg vector («a reflection») where $\mathbf{S}_0$ and $\mathbf{S}$ are direct and diffracted x-ray beams, respectively.

$A(\mathbf{\Delta S})$ are some variables and $\varphi(\mathbf{\Delta S})$ are phases.

A formula of $A(\mathbf{\Delta S})$ depends on the type of Fourier synthesis. In case of difference Fourier synthesis, $A(\mathbf{\Delta S}) = |\, |F_{obs}(\mathbf{\Delta S})| - |F_{calc}(\mathbf{\Delta S})|\, |$ is the difference between observed and calculated values of a structure factor modulus. The first value is the square root of the reflection intensity whereas the second one is calculated from atomic coordinates and thermal parameters, whose values are found and refined using least-square technique in accord with the structural model.

$\varphi(\mathbf{\Delta S})$ is the reflection phase, which can be calculated using known atomic coordinates.

The formula (1) itself does not contain any information on the crystal symmetry what means the result should not depend on that. It is well known, however, that an ideal symmetry correspondence always exists between Fourier maps and structure models. One may suppose that a computational program supports ED calculations based on (1) in a symmetry-independent part of the unit cell. The result is then expanded on the whole cell using the group-symmetry operators. One may assume also that symmetry-averaged $|F|_{obs}$ are used in (1) instead of individual values. It can be finally assumed that both techniques are realized in calculations.

In accordance with arguments presented in [S4], cubic *fcc* symmetry of $LuB_{12}$ crystals is significantly distorted at low temperatures. To provide the ability to derive probable symmetry violations from difference Fourier maps, the crystal structure must be analyzed using a less symmetrical model. Theoretically, one could take P1 symmetry at once. But a positive influence of the intensity average for the symmetry-equivalent groups of reflections is minimized in this case, whereas the influence of other factors (instrumental inaccuracies; non-ideal centering of the crystal in a diffractometer; non-ideal absorption correction and others) becomes stronger. Besides, a redundant symmetry decrease may lead to strong correlations between refined structural parameters. It seems rational, therefore, to start such a research selecting an appropriate symmetry group and take averaged $|F|_{obs}$ for calculations.

Fig. S4 illustrates a symmetry lowering in $LuB_{12}$. X-ray data was collected at T = 140 K using an Xcalibur diffractometer equipped with a CCD detector. In the upper row (panels a-c), difference Fourier maps are presented to elucidate results of the structure refinement in cubic *Fm*-3*m* group. Three planes $z = 0$, $y = 0$, $x = 0$ containing Lu atoms (blue circles) in centers and vertexes of squares (each square is a face of the unit cell) are fully identical down to the smallest details. Green circles are boron sites. Similar Fourier maps in the bottom row (panels d-f) illustrate the structure refinement results in the orthorhombic *Fmmm* group. Boron coordinates are not additionally refined being kept 'cubic' and multiplied by means of one of the rejected three-fold axes. Thermal parameter of Lu is kept isotropic. The only difference is that the residual ED calculations are made from reflections averaged in different point groups (*m*-3*m* or *mmm* for upper and bottom rows, respectively). Three maps differ significantly as a result instead of being equal.

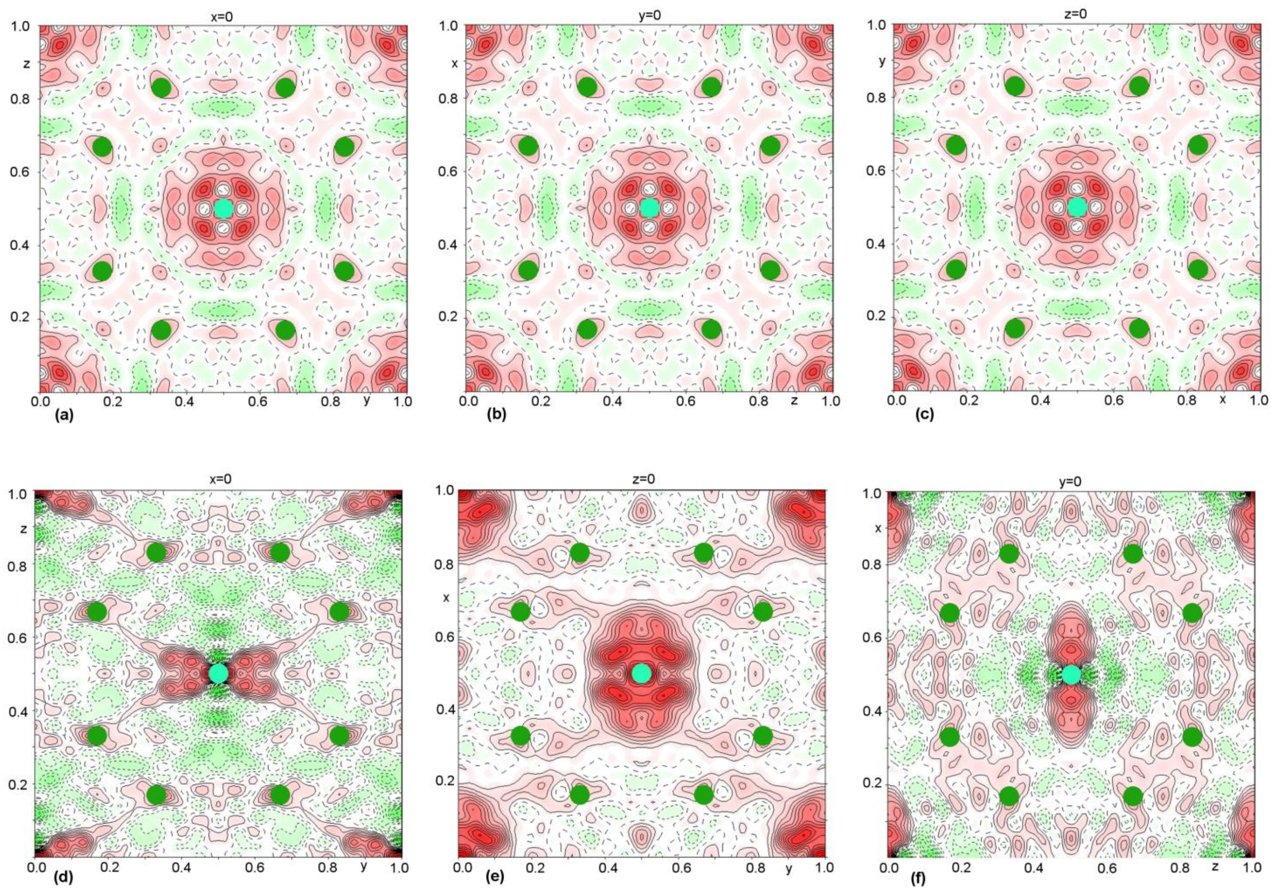


**Fig.S4**. Difference Fourier maps based on the *Fm*-3*m* (a-c) and *Fmmm* (d-f) structure models. Contour intervals are 0.2 e/Å$^3$. Positive (red) and negative (green) residual ED is highlighted.

### Magnetoresistance results in more detail.

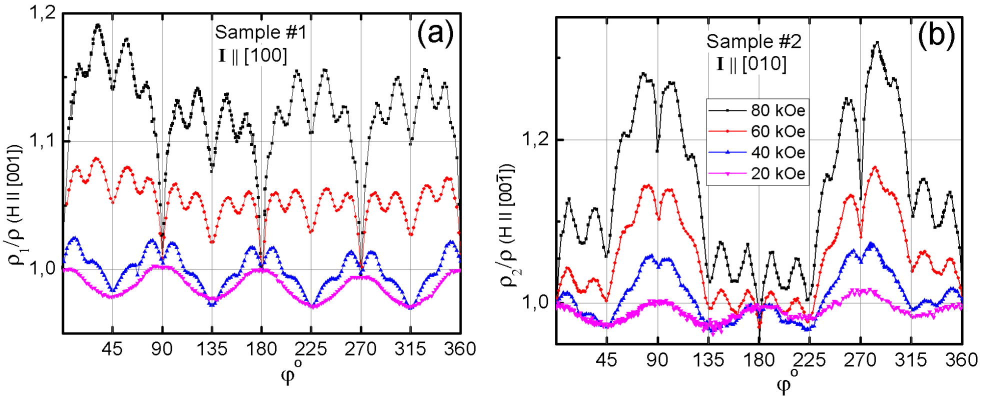


**Fig.S5.** The angular dependences of $\rho(\varphi)$ obtained rotating two crystals of $LuB_{12}$ around the [100] (left panel) and [010] (right panel) axes in various magnetic fields up to 80 kOe at temperature T=2K. Two samples were cut from one single crystalline disc of $LuB_{12}$.

**Quantum chemical results and discussion.** Considering in more detail the possible reasons of the development of the instability of cluster $B_{12}$ it is worth noting, similar to other high-symmetry molecules, that cuboctahedral boron clusters $B_{12}$ may have orbitally-degenerate ground state resulting in JT distortions of the regular cubic structure. In terms of molecular orbitals (MOs), the orbital degeneracy of the ground state is associated with partial electron occupation of the highest occupied molecular orbital (HOMO) of $B_{12}$, which is represented by triply degenerate MOs of t-symmetry. In electrically neutral $[B_{12}]^0$ cluster the HOMO accommodates two electrons ($t^2$ configuration); in negatively charged clusters $[B_{12}]^{n-}$ ($n$ = 1-4) the number $m$ of t-electrons in HOMO increases from three to six (Fig. S6). All electronic configurations $t^m$ with $m$ = 2-5 produce triply degenerate many-electron ground T-state (Fig. S6a-d). This implies that neutral $[B_{12}]^0$ cluster and charged $[B_{12}]^{n-}$ clusters ($n$ = 1, 2, 3) are JT-active systems which would tend to distort cubic structure. Only the $[B_{12}]^{4-}$ cluster with fully occupied HOMO ($t^6$ configuration) has a non-degenerate ground state and thus it is not JT-active (Fig. S6). Specifically, for JT systems with T ground state, two normal vibrational modes of $e$ and $t_2$ symmetry are active, $T\times(e+t_2)$ [S5]. In this case, there are three types of minimum points on the ground potential energy surface of the cubic $T\times(e+t_2)$ JT system, trigonal ($D_{3d}$), tetragonal ($D_{4h}$) and orthorhombic ($D_{2h}$) points. Depending on the ratio between the $e$ and $t_2$ electron-vibronic couplings, either trigonal or tetragonal JT minima can occur, while orthorhombic minima always correspond to the saddle point [S5].

In order to establish the amplitude and type of the JT distortions, we performed quantum chemical calculations and geometry optimizations for the neutral cluster $[B_{12}]^0$ and negatively charged $[B_{12}]^{n-}$ clusters ($n$ = 1-4). Calculations are carried in terms of density functional theory (DFT) using ORCA 3.0.3 quantum chemistry program package at the BP86/def2-SVP level of theory [S6]. In these calculations, the initial point corresponds to the regular $B_{12}$ cuboctahedron and then the structure is allowed to relax freely to reach the local minimum in the potential energy surface. Calculated structures of $[B_{12}]^{n-}$($n$ = 0-4) clusters (Fig. S6) indicate that the JT-active clusters $[B_{12}]^{n-}$($n$ = 0-3) are slightly distorted cuboctahedra. The amplitude and type of JT distortions depends strongly on the charge of the cluster. The neutral cluster and charged clusters with $n$ = 1, 2 exhibit trigonal type of JT distortions, while the $[B_{12}]^{3-}$ cluster shows tetragonal JT distortion. As expected, the non-degenerate $[B_{12}]^{4-}$ cluster has a regular cuboctahedral structure with the $R$(B-B) distance of 1.790 Å (Fig. S6e), which is very close to the experimental value for $LuB_{12}$ (1.787 Å).

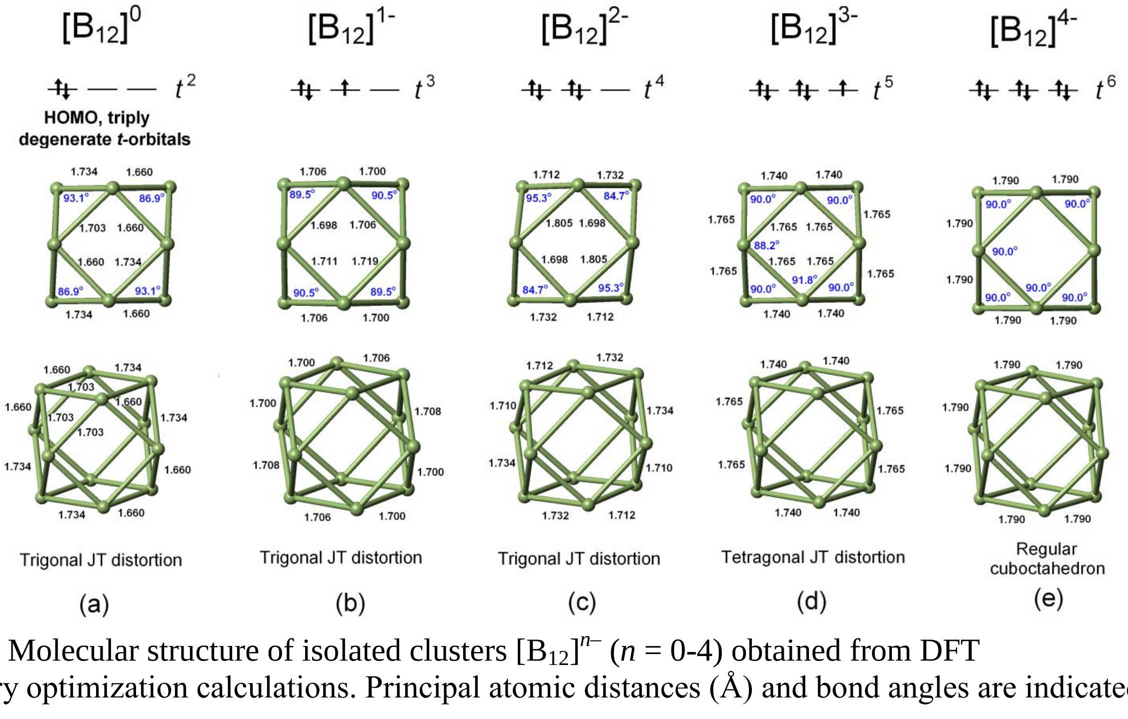


**Fig. S6.** Molecular structure of isolated clusters $[B_{12}]^{n-}$ ($n$ = 0-4) obtained from DFT geometry optimization calculations. Principal atomic distances (Å) and bond angles are indicated.

**References.**

[S1]. A.P. Dudka, I.A. Verin, A.M. Antipin, Crystallography Reports **60**, 316 (2015).

[S2]. I. I. Lobanova, V. V. Glushkov, N. E. Sluchanko, S. V. Demishev, Scientific Reports | 6:22101 | DOI: 10.1038/srep22101 (2016)

[S3]. Petricek, V., Dusek, M. & Palatinus, L. (2014). Z. Kristallogr. 229(5), 345-352. DOI 10.1515/zkri-2014-1737

[S4]. N. B. Bolotina, I. A. Verin, N. Yu. Shitsevalova, V. B. Filippov, and N. E. Sluchanko, Crystallogr. Rep. **61**, 181 (2016).

[S5] I. B. Bersuker, V. Z. Polinger, in Vibronic Interactions in Molecules and Crystals, Springer, Berlin, 1989.

[S6] F. Neese, The ORCA program system, Wiley Interdiscip. Rev.: Comput. Mol. Sci., 2, 73-78 (2012).
